# Supplementary material for: Photoevaporation of Jeans-unstable molecular clumps
Source: arXiv:1905.13230 source file (2019-07-24)
Supplement: Supplementary file 1 [file additional_def.tex]

\def\h2{{\mathrm{H}_2}}

\definecolor{apcolor}{HTML}{b3003b}
\definecolor{afcolor}{HTML}{800080}
\definecolor{ddcolor}{HTML}{077a2f}
